# Supplementary material for: An Empirical Exploration of Trust Dynamics in LLM Supply Chains
Source: arXiv:2405.16310 source file (2024-05-25)
Supplement: Supplementary file 1 [file appendix.tex]

\framedtext{
\textbf{Human entities:}
\begin{itemize}[leftmargin=*]
    \item The space of individual entities: $I$
    \item The space of organizational entities: $O$
    \item Respective instantiations: $i_x \in I$, $o_x \in O$
    \item \textbf{Relations within each human entity type}: $R\_I$, $R\_O$ respectively. 
    \begin{itemize}
        \item These relations are reflexive and symmetric, but not transitive. 
        \item For simplification, we do not specify the type of relation, as it is not important for the exposition of our work. 
    \end{itemize}
    \item \textbf{Relations across human entity types: role}: $R\_IO : I \times O \times type\_IO \rightarrow True / False$    \agathe{TBD: There could be other types of relations between individuals and organizations.  what we do with that when we get to the supply chain relations and "beliefs".}

    \begin{itemize}
        \item The type the relation can take corresponds to the role of the individual entity vis-a-vis the organization. For the purpose of our exposition, we do not need to be exhaustive. We propose for now the following: $type\_IO \in \{None, UX\_researcher, UX\_designer, AI\_researcher, AI\_developer, engineer, product\_manager, legal, governance\}$
        \item Constraints:
        \begin{itemize}
            \item At least one type is always valid per tuple of individual and organization (a role or "None").
            \item One individual can take multiple roles vis-a-vis the same organization, but if so, one of the types cannot be "None".
            \item One individual can have multiple non-"None" type across several organizations (if they work within several organizations). \agathe{TBD whether that's important}
            \item There exists at least always one individual entity that relates to an organization outside the "None" type.
        \end{itemize}
    \end{itemize}
    \item \textbf{Relations between individual entities and technical artifacts}: $R\_ITA: I \times TA \times type\_ITA \rightarrow True/False$
    \begin{itemize}
        \item The type the relation can take corresponds to the type of relation the individual has vis-a-vis the system.
        We propose $type\_ITA = \{impactor, user, potentially\_impacted, public, None\}$
        \item Constraints:
        \begin{itemize}
            \item For technical artifacts of type system, one can assume that there exists always at least one individual entity for each of the possible types in the relation. For technical artifacts of type ``other'', there is at least one individual entity for ``impactor'' and ``user''.
            \item One individual entity can take multiple types vis-a-vis the same AI system.
            \item One individual entity can take multiple types vis-a-vis different AI systems. 
        \end{itemize}
    \end{itemize}
    \item \textbf{Relations between organizational entities and technical artifacts}:  $R\_OTA: O \times TA \times type\_OTA \rightarrow True/False$  
     \begin{itemize}
        \item The type the relation can take corresponds to the type of relation the organization has vis-a-vis the system. 
        We propose $type\_OTA = \{developer, deployer, assessor, user, potentially\_impacted, public, None\}$
        \item Constraints:
        \begin{itemize}
            \item For technical artifacts of type system, on can assume that there exists always at least one organizational entity for each of the possible types in the relation. For technical artifacts of type ``other'', there is at least one organizational entity for ``developer'', ``assessor'', ``deployer'', ``user'' (with the last two having the same meaning).
            \item One organizational entity can take multiple types vis-a-vis the same AI system.
            \item One organizational entity can take multiple types vis-a-vis different AI systems.
        \end{itemize}
    \end{itemize}
    \item Additional constraints: The objective of our work is not to specify in extensive detail the different entities and relations. Yet, we would like to warn the reader (who might want to use our framework) of the existence of additional, obvious, constraints and implications from the relations between the human entities and technical artifacts based on their types. For instance, if an individual entity has the type ``impactor'' vis-a-vis an AI system, then this individual entity should be related to an organization that has a type ``developer'', ``deployer'', or ``assessor'' of the same AI system, and this $R\_IO$ relation should be characterized by a non-"None" type.
    For brevity, we do not describe them further here.
\end{itemize}
}
